# Supplementary material for: A Brief Introduction to Machine Learning for Engineers
Source: arXiv:1709.02840 source file (2018-05-17)
Supplement: Supplementary file 4 [file v_information_measures_from_inference_v11_short_double_column.tex]

%% LyX 2.2.0 created this file.  For more info, see http://www.lyx.org/.
%% Do not edit unless you really know what you are doing.
\documentclass[11pt,two column, english]{IEEEtran}
\usepackage[T1]{fontenc}
\usepackage[latin9]{inputenc}
\usepackage{color}
\usepackage{amsmath}
\usepackage{amssymb}
\linespread{1}

\makeatletter
%%%%%%%%%%%%%%%%%%%%%%%%%%%%%% User specified LaTeX commands.
%% bare_jrnl.tex
%% V1.3
%% 2007/01/11
%% by Michael Shell
%% see http://www.michaelshell.org/
%% for current contact information.
%%
%% This is a skeleton file demonstrating the use of IEEEtran.cls
%% (requires IEEEtran.cls version 1.7 or later) with an IEEE journal paper.
%%
%% Support sites:
%% http://www.michaelshell.org/tex/ieeetran/
%% http://www.ctan.org/tex-archive/macros/latex/contrib/IEEEtran/
%% and
%% http://www.ieee.org/



% *** Authors should verify (and, if needed, correct) their LaTeX system  ***
% *** with the testflow diagnostic prior to trusting their LaTeX platform ***
% *** with production work. IEEE's font choices can trigger bugs that do  ***
% *** not appear when using other class files.                            ***
% The testflow support page is at:
% http://www.michaelshell.org/tex/testflow/


%%*************************************************************************
%% Legal Notice:
%% This code is offered as-is without any warranty either expressed or
%% implied; without even the implied warranty of MERCHANTABILITY or
%% FITNESS FOR A PARTICULAR PURPOSE!
%% User assumes all risk.
%% In no event shall IEEE or any contributor to this code be liable for
%% any damages or losses, including, but not limited to, incidental,
%% consequential, or any other damages, resulting from the use or misuse
%% of any information contained here.
%%
%% All comments are the opinions of their respective authors and are not
%% necessarily endorsed by the IEEE.
%%
%% This work is distributed under the LaTeX Project Public License (LPPL)
%% ( http://www.latex-project.org/ ) version 1.3, and may be freely used,
%% distributed and modified. A copy of the LPPL, version 1.3, is included
%% in the base LaTeX documentation of all distributions of LaTeX released
%% 2003/12/01 or later.
%% Retain all contribution notices and credits.
%% ** Modified files should be clearly indicated as such, including  **
%% ** renaming them and changing author support contact information. **
%%
%% File list of work: IEEEtran.cls, IEEEtran_HOWTO.pdf, bare_adv.tex,
%%                    bare_conf.tex, bare_jrnl.tex, bare_jrnl_compsoc.tex
%%*************************************************************************
% Note that the a4paper option is mainly intended so that authors in
% countries using A4 can easily print to A4 and see how their papers will
% look in print - the typesetting of the document will not typically be
% affected with changes in paper size (but the bottom and side margins will).
% Use the testflow package mentioned above to verify correct handling of
% both paper sizes by the user's LaTeX system.
% Also note that the "draftcls" or "draftclsnofoot", not "draft", option
% should be used if it is desired that the figures are to be displayed in
% draft mode.
% If IEEEtran.cls has not been installed into the LaTeX system files,
% manually specify the path to it like:
% \documentclass[journal]{../sty/IEEEtran}





% Some very useful LaTeX packages include:
% (uncomment the ones you want to load)


% *** MISC UTILITY PACKAGES ***
%\usepackage{ifpdf}
% Heiko Oberdiek's ifpdf.sty is very useful if you need conditional
% compilation based on whether the output is pdf or dvi.
% usage:
% \ifpdf
%   % pdf code
% \else
%   % dvi code
% \fi
% The latest version of ifpdf.sty can be obtained from:
% http://www.ctan.org/tex-archive/macros/latex/contrib/oberdiek/
% Also, note that IEEEtran.cls V1.7 and later provides a builtin
% \ifCLASSINFOpdf conditional that works the same way.
% When switching from latex to pdflatex and vice-versa, the compiler may
% have to be run twice to clear warning/error messages.






% *** CITATION PACKAGES ***
%\usepackage{cite}
% cite.sty was written by Donald Arseneau
% V1.6 and later of IEEEtran pre-defines the format of the cite.sty package
% \cite{} output to follow that of IEEE. Loading the cite package will
% result in citation numbers being automatically sorted and properly
% "compressed/ranged". e.g., [1], [9], [2], [7], [5], [6] without using
% cite.sty will become [1], [2], [5]--[7], [9] using cite.sty. cite.sty's
% \cite will automatically add leading space, if needed. Use cite.sty's
% noadjust option (cite.sty V3.8 and later) if you want to turn this off.
% cite.sty is already installed on most LaTeX systems. Be sure and use
% version 4.0 (2003-05-27) and later if using hyperref.sty. cite.sty does
% not currently provide for hyperlinked citations.
% The latest version can be obtained at:
% http://www.ctan.org/tex-archive/macros/latex/contrib/cite/
% The documentation is contained in the cite.sty file itself.






% *** GRAPHICS RELATED PACKAGES ***
\ifCLASSINFOpdf% \usepackage[pdftex]{graphicx}
% declare the path(s) where your graphic files are
% \graphicspath{{../pdf/}{../jpeg/}}
% and their extensions so you won't have to specify these with
% every instance of \includegraphics
% \DeclareGraphicsExtensions{.pdf,.jpeg,.png}
\else% or other class option (dvipsone, dvipdf, if not using dvips). graphicx
% will default to the driver specified in the system graphics.cfg if no
% driver is specified.
% \usepackage[dvips]{graphicx}
% declare the path(s) where your graphic files are
% \graphicspath{{../eps/}}
% and their extensions so you won't have to specify these with
% every instance of \includegraphics
% \DeclareGraphicsExtensions{.eps}
\fi% graphicx was written by David Carlisle and Sebastian Rahtz. It is
% required if you want graphics, photos, etc. graphicx.sty is already
% installed on most LaTeX systems. The latest version and documentation can
% be obtained at:
% http://www.ctan.org/tex-archive/macros/latex/required/graphics/
% Another good source of documentation is "Using Imported Graphics in
% LaTeX2e" by Keith Reckdahl which can be found as epslatex.ps or
% epslatex.pdf at: http://www.ctan.org/tex-archive/info/
% latex, and pdflatex in dvi mode, support graphics in encapsulated
% postscript (.eps) format. pdflatex in pdf mode supports graphics
% in .pdf, .jpeg, .png and .mps (metapost) formats. Users should ensure
% that all non-photo figures use a vector format (.eps, .pdf, .mps) and
% not a bitmapped formats (.jpeg, .png). IEEE frowns on bitmapped formats
% which can result in "jaggedy"/blurry rendering of lines and letters as
% well as large increases in file sizes.
% You can find documentation about the pdfTeX application at:
% http://www.tug.org/applications/pdftex





% *** MATH PACKAGES ***
%\usepackage[cmex10]{amsmath}
% A popular package from the American Mathematical Society that provides
% many useful and powerful commands for dealing with mathematics. If using
% it, be sure to load this package with the cmex10 option to ensure that
% only type 1 fonts will utilized at all point sizes. Without this option,
% it is possible that some math symbols, particularly those within
% footnotes, will be rendered in bitmap form which will result in a
% document that can not be IEEE Xplore compliant!
% Also, note that the amsmath package sets \interdisplaylinepenalty to 10000
% thus preventing page breaks from occurring within multiline equations. Use:
%\interdisplaylinepenalty=2500
% after loading amsmath to restore such page breaks as IEEEtran.cls normally
% does. amsmath.sty is already installed on most LaTeX systems. The latest
% version and documentation can be obtained at:
% http://www.ctan.org/tex-archive/macros/latex/required/amslatex/math/





% *** SPECIALIZED LIST PACKAGES ***
%\usepackage{algorithmic}
% algorithmic.sty was written by Peter Williams and Rogerio Brito.
% This package provides an algorithmic environment fo describing algorithms.
% You can use the algorithmic environment in-text or within a figure
% environment to provide for a floating algorithm. Do NOT use the algorithm
% floating environment provided by algorithm.sty (by the same authors) or
% algorithm2e.sty (by Christophe Fiorio) as IEEE does not use dedicated
% algorithm float types and packages that provide these will not provide
% correct IEEE style captions. The latest version and documentation of
% algorithmic.sty can be obtained at:
% http://www.ctan.org/tex-archive/macros/latex/contrib/algorithms/
% There is also a support site at:
% http://algorithms.berlios.de/index.html
% Also of interest may be the (relatively newer and more customizable)
% algorithmicx.sty package by Szasz Janos:
% http://www.ctan.org/tex-archive/macros/latex/contrib/algorithmicx/




% *** ALIGNMENT PACKAGES ***
%\usepackage{array}
% Frank Mittelbach's and David Carlisle's array.sty patches and improves
% the standard LaTeX2e array and tabular environments to provide better
% appearance and additional user controls. As the default LaTeX2e table
% generation code is lacking to the point of almost being broken with
% respect to the quality of the end results, all users are strongly
% advised to use an enhanced (at the very least that provided by array.sty)
% set of table tools. array.sty is already installed on most systems. The
% latest version and documentation can be obtained at:
% http://www.ctan.org/tex-archive/macros/latex/required/tools/


%\usepackage{mdwmath}
%\usepackage{mdwtab}
% Also highly recommended is Mark Wooding's extremely powerful MDW tools,
% especially mdwmath.sty and mdwtab.sty which are used to format equations
% and tables, respectively. The MDWtools set is already installed on most
% LaTeX systems. The lastest version and documentation is available at:
% http://www.ctan.org/tex-archive/macros/latex/contrib/mdwtools/


% IEEEtran contains the IEEEeqnarray family of commands that can be used to
% generate multiline equations as well as matrices, tables, etc., of high
% quality.


%\usepackage{eqparbox}
% Also of notable interest is Scott Pakin's eqparbox package for creating
% (automatically sized) equal width boxes - aka "natural width parboxes".
% Available at:
% http://www.ctan.org/tex-archive/macros/latex/contrib/eqparbox/





% *** SUBFIGURE PACKAGES ***
%\usepackage[tight,footnotesize]{subfigure}
% subfigure.sty was written by Steven Douglas Cochran. This package makes it
% easy to put subfigures in your figures. e.g., "Figure 1a and 1b". For IEEE
% work, it is a good idea to load it with the tight package option to reduce
% the amount of white space around the subfigures. subfigure.sty is already
% installed on most LaTeX systems. The latest version and documentation can
% be obtained at:
% http://www.ctan.org/tex-archive/obsolete/macros/latex/contrib/subfigure/
% subfigure.sty has been superceeded by subfig.sty.



%\usepackage[caption=false]{caption}
%\usepackage[font=footnotesize]{subfig}
% subfig.sty, also written by Steven Douglas Cochran, is the modern
% replacement for subfigure.sty. However, subfig.sty requires and
% automatically loads Axel Sommerfeldt's caption.sty which will override
% IEEEtran.cls handling of captions and this will result in nonIEEE style
% figure/table captions. To prevent this problem, be sure and preload
% caption.sty with its "caption=false" package option. This is will preserve
% IEEEtran.cls handing of captions. Version 1.3 (2005/06/28) and later
% (recommended due to many improvements over 1.2) of subfig.sty supports
% the caption=false option directly:
%\usepackage[caption=false,font=footnotesize]{subfig}
% The latest version and documentation can be obtained at:
% http://www.ctan.org/tex-archive/macros/latex/contrib/subfig/
% The latest version and documentation of caption.sty can be obtained at:
% http://www.ctan.org/tex-archive/macros/latex/contrib/caption/




% *** FLOAT PACKAGES ***
%\usepackage{fixltx2e}
% fixltx2e, the successor to the earlier fix2col.sty, was written by
% Frank Mittelbach and David Carlisle. This package corrects a few problems
% in the LaTeX2e kernel, the most notable of which is that in current
% LaTeX2e releases, the ordering of single and double column floats is not
% guaranteed to be preserved. Thus, an unpatched LaTeX2e can allow a
% single column figure to be placed prior to an earlier double column
% figure. The latest version and documentation can be found at:
% http://www.ctan.org/tex-archive/macros/latex/base/



%\usepackage{stfloats}
% stfloats.sty was written by Sigitas Tolusis. This package gives LaTeX2e
% the ability to do double column floats at the bottom of the page as well
% as the top. (e.g., "\begin{figure*}[!b]" is not normally possible in
% LaTeX2e). It also provides a command:
%\fnbelowfloat
% to enable the placement of footnotes below bottom floats (the standard
% LaTeX2e kernel puts them above bottom floats). This is an invasive package
% which rewrites many portions of the LaTeX2e float routines. It may not work
% with other packages that modify the LaTeX2e float routines. The latest
% version and documentation can be obtained at:
% http://www.ctan.org/tex-archive/macros/latex/contrib/sttools/
% Documentation is contained in the stfloats.sty comments as well as in the
% presfull.pdf file. Do not use the stfloats baselinefloat ability as IEEE
% does not allow \baselineskip to stretch. Authors submitting work to the
% IEEE should note that IEEE rarely uses double column equations and
% that authors should try to avoid such use. Do not be tempted to use the
% cuted.sty or midfloat.sty packages (also by Sigitas Tolusis) as IEEE does
% not format its papers in such ways.


%\ifCLASSOPTIONcaptionsoff
%  \usepackage[nomarkers]{endfloat}
% \let\MYoriglatexcaption\caption
% \renewcommand{\caption}[2][\relax]{\MYoriglatexcaption[#2]{#2}}
%\fi
% endfloat.sty was written by James Darrell McCauley and Jeff Goldberg.
% This package may be useful when used in conjunction with IEEEtran.cls'
% captionsoff option. Some IEEE journals/societies require that submissions
% have lists of figures/tables at the end of the paper and that
% figures/tables without any captions are placed on a page by themselves at
% the end of the document. If needed, the draftcls IEEEtran class option or
% \CLASSINPUTbaselinestretch interface can be used to increase the line
% spacing as well. Be sure and use the nomarkers option of endfloat to
% prevent endfloat from "marking" where the figures would have been placed
% in the text. The two hack lines of code above are a slight modification of
% that suggested by in the endfloat docs (section 8.3.1) to ensure that
% the full captions always appear in the list of figures/tables - even if
% the user used the short optional argument of \caption[]{}.
% IEEE papers do not typically make use of \caption[]'s optional argument,
% so this should not be an issue. A similar trick can be used to disable
% captions of packages such as subfig.sty that lack options to turn off
% the subcaptions:
% For subfig.sty:
% \let\MYorigsubfloat\subfloat
% \renewcommand{\subfloat}[2][\relax]{\MYorigsubfloat[]{#2}}
% For subfigure.sty:
% \let\MYorigsubfigure\subfigure
% \renewcommand{\subfigure}[2][\relax]{\MYorigsubfigure[]{#2}}
% However, the above trick will not work if both optional arguments of
% the \subfloat/subfig command are used. Furthermore, there needs to be a
% description of each subfigure *somewhere* and endfloat does not add
% subfigure captions to its list of figures. Thus, the best approach is to
% avoid the use of subfigure captions (many IEEE journals avoid them anyway)
% and instead reference/explain all the subfigures within the main caption.
% The latest version of endfloat.sty and its documentation can obtained at:
% http://www.ctan.org/tex-archive/macros/latex/contrib/endfloat/
% The IEEEtran \ifCLASSOPTIONcaptionsoff conditional can also be used
% later in the document, say, to conditionally put the References on a
% page by themselves.





% *** PDF, URL AND HYPERLINK PACKAGES ***
%\usepackage{url}
% url.sty was written by Donald Arseneau. It provides better support for
% handling and breaking URLs. url.sty is already installed on most LaTeX
% systems. The latest version can be obtained at:
% http://www.ctan.org/tex-archive/macros/latex/contrib/misc/
% Read the url.sty source comments for usage information. Basically,
% \url{my_url_here}.





% *** Do not adjust lengths that control margins, column widths, etc. ***
% *** Do not use packages that alter fonts (such as pslatex).         ***
% There should be no need to do such things with IEEEtran.cls V1.6 and later.
% (Unless specifically asked to do so by the journal or conference you plan
% to submit to, of course. )


% correct bad hyphenation here
%\hyphenation{op-tical net-works semi-conduc-tor}
%\makeatother
\usepackage{babel}




%\makeatother
%\usepackage{babel}



\usepackage{babel}

\makeatother

\usepackage{babel}
\begin{document}
% paper title
% can use linebreaks \\ within to get better formatting as desired

\title{Introducing Information Measures via Inference {[}Lecture Notes{]}}

\author{Osvaldo Simeone}

\maketitle
\vspace{-50pt}
Information measures, such as the entropy and the Kullback-Leibler
(KL) divergence, are typically introduced in Information Theory, Pattern
Recognition and Machine Learning books using an abstract viewpoint
based on a notion of ``surprise'': the entropy of a given random
variable is larger if its realization, when revealed, is on average
more ``surprising'' (see, e.g., \cite{Cover,Bishop}). The goal of
these lecture notes is to describe a principled and intuitive introduction
to information measures that builds on inference, namely estimation
and hypothesis testing. Specifically, entropy and conditional entropy
measures are defined using variational characterizations that can
be interpreted in terms of the minimum Bayes risk in an estimation
problem. Divergence metrics are similarly described using variational
expressions derived via mismatched estimation or binary hypothesis
testing principles. The classical Shannon entropy and the KL divergence
are recovered as special cases of more general families of information
measures. 
\vspace{-15pt}
\subsection*{Relevance}

Information measures are among the criteria most commonly used to
derive pattern recognition and machine learning methods, including
blind source separation and variational inference. An understanding
of information measures in terms of inference principles can clarify
their significance and illuminate the implications of their adoption
for signal processing and learning problems. 
\vspace{-15pt}
\subsection*{Prerequisites}

These notes require basic knowledge in probability and statistics.

\section*{Problem Statement}

We consider the following three questions.\\
\indent 1. Given a random variable $X$ distributed according to a known probabilistic model $p_{X}(x)$, i.e., $X\sim p_{X}$, how can
we measure the information associated with its observation? Addressing
this question leads to the definition of generalized entropy as the
minimum average loss, or Bayes risk, attainable on the estimate of
$X$ based only on the knowledge of the probabilistic model $p_{X}$
\cite{GrunwaldDawid}. \\
\indent 2. Given two random variables $X$ and $Y$ jointly distributed according
to a known probabilistic model $p_{XY}(x,y)$, i.e., $(X,Y)\sim p_{XY}$,
how can we measure the information associated with the observation
of $X$ when $Y$ is already known? This leads to the definition of
the generalized conditional entropy as the minimum average loss, or
Bayes risk, attainable on the estimate of $X$ given the knowledge
of $Y$ and of the probabilistic model $p_{XY}$ \cite{GrunwaldDawid}. \\
\indent 3. Given two probabilistic models $p_{X}$ and $q_{X}$ defined over
the same alphabet $\mathcal{X}$, how can we quantify how ``different''
they are? Tackling this question leads to the definition of divergence
measures, such as the KL divergence, based on either mismatched estimation
\cite{GrunwaldDawid,Farnia} or binary hypothesis testing \cite{Jordan,fgan}
principles. \\
\indent Throughout these notes, we focus on the case of discrete random variables
taking values in finite alphabets indicated by calligraphic letters,
as in $X\in\mathcal{X}$ for a random variable $X$. For extensions
to more general alphabets, we refer to the bibliography. We will denote
to the probability mass function (pmf) of a discrete random variable
$X$ as $p_{X}$. The conditional pmf of $X$ given the observation
$Y=y$ of a jointly distributed random variable $Y$ is indicated
as $p_{X|Y=y}$, so that $p_{X|Y}$ is a random pmf indexed by $Y$.
The notation $E_{X\sim p_{X}}[\cdot]$ indicates the expectation of
the argument with respect to the random variable $X\sim p_{X}$, and the conditional expectation is defined in a similar way. $\textrm{var}(\cdot)$
represents the variance of the argument pmf. The notation $\log$
represents the logarithm in base two.

\section*{Solution}

\subsection*{\textcolor{black}{1. Generalized Entropy}}

As proposed by Claude Shannon, the amount of information received
from the observation of a discrete random variable $X\sim p_{X}(x)$
defined over a finite alphabet $\mathcal{X}$ should be measured by
the amount of a uncertainty about its value prior to its measurement
\cite{Shannon}. This is typically done by introducing the ``surprise''
associated with the occurrence of an outcome $x$ as $-\textrm{log}_{2}p_{X}(x)$,
which is indeed an increasing function of $p_{X}(x)^{-1}$ \textendash{}
the more unlikely $x$ is, the larger is its induced surprise. The
average surprise is the Shannon entropy 
\begin{equation}
H(X)=\textrm{E}_{X\sim p_{X}}[-\textrm{log}p_{X}(X)].\label{eq:Shannon entropy}
\end{equation}
The logarithmic surprise measure $-\textrm{log}p_{X}(x)$ can be justified
based on engineering arguments as well as by using an axiomatic approach
\cite{Shannon}. 

Taking a step back, we would like to outline a more direct approach
for quantifying the information associated with the observation of a random
variable $X$. To this end, we consider the problem of estimating the
value of $X$ when one only knows the probabilistic model $p_{X}$.
The key idea is that the observation of a random variable $X$ is
more informative if its value is more difficult to predict a priori,
that is, based only on the knowledge of $p_{X}$. 

To formalize this notion, we need to specify: (\emph{i}) the type
of estimates that one is allowed to make on the value of $X$; and
(\emph{ii}) the loss function $\ell$ that is used to measure the
accuracy of the estimate. We will proceed by considering two types
of estimates, namely \emph{point estimates}, whereby one needs to
commit to a specific value $\hat{x}\in\mathcal{X}$ as the estimate
of $X$; and \emph{distributional estimates}, in which instead we
are allowed to produce a pmf $\hat{p}_{X}(x)$ over alphabet $\mathcal{X}$,
hence defining a profile of "beliefs" over the possible values of $X$.

\emph{Point Estimates}: Given a point estimate $\hat{x}\in\mathcal{X}$
and an observed value $x\in\mathcal{X}$, the estimation error can
be measured by a non-negative loss function $\ell(x,\hat{x})$. Examples
include the quadratic loss function $\ell_{2}(x,\hat{x})=(x-\hat{x})^{2}$;
and the 0-1 loss function, or detection error, $\ell_{0}(x,\hat{x})=|x-\hat{x}|_{0},$
where $|a|_{0}=0$ if $a=0$ and $|a|_{0}=1$ otherwise. For any
given loss function $\ell$, based on the discussion above, we can
measure the information accrued by the observation of $X\sim p_{X}$
by evaluating the average loss that is incurred by the best possible
a priori estimate of $X$. This leads to the definition of generalized
entropy \cite{GrunwaldDawid} 
\begin{equation}
H_{\ell}(X)=H_{\ell}(p_{X})=\min_{\hat{x}}\textrm{E\ensuremath{_{X\sim p_{X}}}[}\ell(X,\hat{x})],\label{eq:generalized entropy definition}
\end{equation}
where the estimate $\hat{x}$ is not constrained to lie in the alphabet
$\mathcal{X}$. As highlighted by the notation $H_{\ell}(p_{X})$,
the generalized entropy depends on the pmf $p_{X}$ and on the loss
function $\ell$. The notion of generalized entropy (\ref{eq:generalized entropy definition})
coincides with that of minimum Bayes risk for the given loss function
$\ell$. 

Let us consider the examples of the quadratic and 0-1 loss functions.
For the former, the generalized entropy can be computed as 
\begin{align}
H_{\ell_{2}}(p_{X})=\textrm{var}(p_{X}),
\end{align}
where we have imposed the optimality condition $\textrm{d}\textrm{E[}(X-\hat{x})^{2}]/\textrm{d}\hat{x}=0$
to conclude that the optimal point estimate is the mean $\hat{x}=\textrm{E}_{X\sim p_X}[X].$
Under the quadratic loss function, the generalized entropy is hence simply
the variance of the distribution. As for the 0-1 loss, we can write
\begin{equation}
H_{\ell_{0}}(p_{X})=\min_{\hat{x}}\sum_{x\neq\hat{x}}p_{X}(x)=1-\max_{\hat{x}}p_{X}(\hat{x}),\label{eq:gen entropy 0}
\end{equation}
since the optimal estimate is the mode, i.e., the value $\hat{x}$
with the largest probability $p_{X}(\hat{x})$. The generalized entropy (\ref{eq:gen entropy 0})
equals the minimum probability of error for the detection of $X$.

\emph{Distributional Estimate: }We now consider a different type of
estimation problem in which we are permitted to choose a pmf $\hat{p}_{X}(x)$
on the alphabet $\mathcal{X}$ as the estimate for the outcome of
variable $X$. To ease intuition, we can imagine $\hat{p}_{X}(x)$
to represent the fraction of one's wager that is invested on the outcome
of $X$ being a specific value $x$. Note that it may not be necessarily
optimal to put all of one's money on one value $x$!
In fact, this depends on how we measure the reward, or conversely
the cost, obtained when a value $x$ is realized.

To this end, we define a non-negative loss function $\ell(x,\hat{p}_{X})$
representing the loss, or the ``negative gain'', suffered when the
value $x$ is observed. This loss should sensibly be a decreasing
function of $\hat{p}_{X}(x)$ \textendash{} we register a smaller
loss, or conversely a larger gain, when we have wagered more on the
actual outcome $x$. As a fairly general class of loss functions,
we can hence define 
\begin{equation}
\ell(x,\hat{p}_{X})=f(\hat{p}_{X}(x)),\label{eq:loss distributional}
\end{equation}
where $f$ is a decreasing function. More general classes of loss functions
are considered in \cite{Ruan}.

Denote as $\Delta(\mathcal{X})$ the simplex of pmfs defined over
alphabet $\mathcal{X}$. The generalized entropy can now be defined
in a way that is formally equivalent to (\ref{eq:generalized entropy definition}),
with the only difference being the optimization over pmf $\hat{p}_{X}$
rather than over point estimate $\hat{x}$: 
\begin{equation}
H_{\ell}(X)=H_{\ell}(p_{X})=\min_{\hat{p}_{X}\in\Delta(\mathcal{X})}\textrm{E\ensuremath{_{X\sim p_{X}}}[}\ell(X,\hat{p}_{X})].\label{eq:generalized entropy definition-1}
\end{equation}

A key example of loss function $\ell(x,\hat{p}_{X})$ in class (\ref{eq:loss distributional})
is the \emph{log-loss} $\ell(x,\hat{p}_{X})=-\log\hat{p}_{X}(x)$.
The log-loss has a strong motivation in terms of lossless compression.
In fact, by Kraft's inequality \cite{Cover}, it is possible to design
a prefix-free \textendash{} and hence decodable without delay \textendash{}
lossless compression scheme that uses $\left\lceil -\log\hat{p}_{X}(x)\right\rceil $
bits to represent value $x$. As a result, the choice of a pmf $\hat{p}_{X}$
is akin to the selection of a prefix-free lossless compression scheme
that requires a description of around $-\log\hat{p}_{X}(x)$ bits to
represent value $x$. The expectation in (\ref{eq:generalized entropy definition-1})
measures the corresponding average number of bits required for lossless
compression by the given scheme.

Using the log-loss in (\ref{eq:generalized entropy definition}),
we obtain 
\begin{equation}
H(p_{X})=\min_{\hat{p}_{X}\in\Delta(\mathcal{X})}\textrm{E\ensuremath{_{X\sim p_{X}}}\ensuremath{[-}\ensuremath{\log}\ensuremath{\ensuremath{\hat{p}_{X}}(x)}}],\label{eq:Shannon as log loss}
\end{equation}
where $H(p_{X})$ is the Shannon entropy (\ref{eq:Shannon entropy}).
In fact, imposing the optimality condition yields the optimal pmf $\hat{p}_{X}(x)$
as $\hat{p}_{X}(x)=p_{X}(x)$. Equation (\ref{eq:Shannon as log loss}) reveals that the entropy (\ref{eq:Shannon entropy})
is the minimum average log-loss when optimizing over all possible
pmfs $\hat{p}_{X}$. 

It may seem at first glance that the choice $\hat{p}_{X}(x)=p_{X}(x)$
should be optimal for most reasonable loss functions in class (\ref{eq:loss distributional}), but this is not the case. In fact,
when the alphabet $\mathcal{X}$ has more than two elements, it can
be proved that the log-loss \textendash{} more generally defined as
$\ell(x,\hat{p}_{X})=b\log\hat{p}_{X}(x)+c$ with $b\leq0$ and any
$c$ \textendash{} is the only loss function of the form (\ref{eq:loss distributional})
for which $\hat{p}_{X}(x)=p_{X}(x)$ is optimal \cite[Theorem 1]{Jiao}.

\emph{Remark}: When $p_{X}$ is the empirical distribution of the
data and the optimization over the pmf $\hat{p}_{X}$ is constrained
to lie in a given set of parametrized pmfs, the cost function in (\ref{eq:Shannon as log loss})
is typically referred to as the \emph{cross-entropy} loss and the
resulting problem coincides with the Maximum Likelihood (ML) estimation of the parametrized
model $\hat{p}_{X}$ \cite{Bishop}.

\emph{Remark: }The generalized entropy $H_{\ell}(p_{X})$ is a concave
function of $p_{X}$, which means that we have the inequality $H_{\ell}(\lambda p_{X}+(1-\lambda)q_{X})\geq\lambda H_{\ell}(p_{X})+(1-\lambda)H_{\ell}(q_{X})$
for any two distributions $p_{X}$ and $q_{X}$ and any $0\leq\lambda\leq1$.
This follows from the fact that the entropy is the minimum over a
family of linear functionals of $p_{X}$ \cite{Boyd}. The concavity of $H_{\ell}(p_{X})$
implies that a variable $X\sim\lambda p_{X}+(1-\lambda)q_{X}$ distributed
according to the mixture of two distributions is more ``random'',
i.e., it is more difficult to estimate, than both variables $X\sim p_{X}$
and $Y\sim q_{X}$. 

\subsection*{2. Generalized Conditional Entropy and Mutual Information}

Given two random variables $X$ and $Y$ jointly distributed according
to a known probabilistic model $p_{XY}(x,y)$, i.e., $(X,Y)\sim p_{XY}$,
we now discuss how to quantify the information that the observation
of one variable, say $Y$, brings about the other, namely $X$. Following
the same approach adopted above, we can distinguish two inferential
scenarios for this purpose: in the first, a point estimate $\hat{x}(y)$
of $X$ needs to be produced based on the observation of a value $Y=y$
and the knowledge of the joint pmf $p_{XY}$; while, in the second,
we are allowed to choose a pmf $\hat{p}_{X|Y=y}$ as the estimate
of $X$ given the observation $Y=y.$

\emph{Point Estimate}: Assuming point estimates and given a loss function
$\ell(x,\hat{x})$, the generalized conditional entropy for an observation
$Y=y$ is defined as the minimum average loss
\begin{equation}
H_{\ell}(p_{X|Y=y})=\min_{\hat{x}(y)\in\mathcal{X}}\textrm{E\ensuremath{_{X\sim p_{X|Y=y}}}[}\ell(X,\hat{x}(y))|Y=y].\label{eq:generalized conditional entropy}
\end{equation}
Note that this definition is consistent with (\ref{eq:generalized conditional entropy})
as applied to the conditional pmf $p_{X|Y=y}$. Averaging over the
distribution of the observation $Y$ yields the generalized conditional
entropy 
\begin{equation}
H_{\ell}(X|Y)=\textrm{E}_{Y\sim p_{Y}}[H_{\ell}(p_{X|Y})].\label{eqgeneratlized conditional entropy 1}
\end{equation}
It is emphasized that the generalized conditional entropy depends
on the joint distribution $p_{XY}$, while (\ref{eq:generalized conditional entropy})
depends only on the conditional pmf $p_{X|Y=y}$.

For the squared error, the entropy can be easily seen to be the
average conditional variance $H_{\ell_{2}}(X|Y)=\textrm{E}_{Y\sim p_{Y}}[\textrm{var}$$(p_{X|Y})${]},
since the a posteriori mean $\hat{x}(y)=\textrm{E}_{X\sim p_{X|Y=y}}[X|Y=y]$
is the optimal estimate. For the 0-1 loss, the generalized conditional
entropy $H_{\ell_{0}}(X|Y)$ is instead equal to the minimum probability of error for the detection of $X$
given $Y$ and the maximum a posteriori (MAP) estimate $\hat{x}(y)=\textrm{argmax}_{\hat{x}\in\mathcal{X}}p_{X|Y}(\hat{x}|y)$
is optimal. 

\emph{Distributional Estimate}: Assume now that we are allowed to
choose a pmf $\hat{p}_{X|Y=y}$ as the estimate of $X$ given the
observation $Y=y$, and that we measure the estimation loss via a
function $\ell(x,\hat{p}_{X})$ as in (\ref{eq:loss distributional}).
The definition of generalized conditional entropy for a given value
of $Y=y$ follows directly from the arguments above and is given as $H_{\ell}(p_{X|Y=y})$, while the generalized conditional entropy is (\ref{eqgeneratlized conditional entropy 1}).
With the log-loss function, the definition above can be again seen to coincide
with Shannon conditional entropy $H(X|Y)=\textrm{E\ensuremath{_{X,Y\sim p_{X,Y}}}[}-\textrm{log}p_{X|Y}(X)]$. 

\emph{Remark}: If $X$ and $Y$ are independent, we have the equality
$H_{\ell}(X|Y)=H_{\ell}(X)$. Furthermore, since in (\ref{eq:generalized conditional entropy})
we can always choose
estimates that are independent of $Y$, we generally have the inequality
$H_{\ell}(X|Y)\leq H_{\ell}(X)$: observing $Y$, on average, can
only decrease the entropy. Note, however, that it is not true that
$H_{\ell}(p_{X|Y=y})$ is necessarily smaller than $H_{\ell}(X)$ \cite[Chapter 2]{Cover}.

\emph{Remark}: Assume that $p_{X,Y}$ is the empirical distribution of the
data, typically referred to as domain variables $X$ and labels $Y$, and that the optimization
over the conditional pmf $\hat{p}_{X|Y}$ is constrained to lie in a
given set of parametrized pmfs. In this case, the cost function $\textrm{E\ensuremath{_{X,Y\sim p_{X,Y}}}[}-\textrm{log}\hat{p}_{X|Y}(X)]$
is again defined as the cross-entropy loss, and the resulting problem
coincides with the ML supervised learning of the parametrized model
$\hat{p}_{X|Y}$, as in, e.g., logistic regression \cite{Bishop}.

\emph{Mutual Information}: The inequality $H_{\ell}(X|Y)\leq H_{\ell}(X)$ justifies
the definition of generalized mutual information with respect to
the given loss function $\ell$ as
\begin{equation}
I_{\ell}(X;Y)=H_{\ell}(X)-H_{\ell}(X|Y).\label{eq:mutual information}
\end{equation}
The mutual information measures the decrease in average loss that is obtained by observing $Y$ as compared to having only prior information about $p_X$. This notion of mutual information is in line with the concept of statistical information proposed by DeGroot (see \cite{Ruan} for a recent treatment). With the log-loss, the generalized mutual information (\ref{eq:mutual information}) reduces to Shannon's mutual information. 

\subsection*{3. Divergence Measures}

Here we discuss how to quantify the ``difference'' between two given
probabilistic models $p_{X}$ and $q_{X}$ defined over the same alphabet
$\mathcal{X}.$ We will take two different viewpoints that will lead
to different definitions of divergence between two distributions.
The first is based on mismatched inference and follows naturally the
approach used above to define generalized entropy, conditional entropy and mutual
information; while the second is based on the conceptually distinct
inferential scenario of binary hypothesis testing.

\emph{Mismatched Inference}: Assume that the correct probabilistic
model $p_{X}$, from which the observation $X\sim p_{X}$ is drawn,
is not known, but only an approximation $q_{X}$ is available. The
point estimate $\hat{x}$ can hence depend only on $q_{X}$, and is
selected by minimizing the mismatched average loss as \begin{equation}
\hat{x}^{(q_{X})}=\textrm{argmin\ensuremath{_{\hat{x}\in\mathcal{X}}}}\textrm{E}_{X\sim q_{X}}[\ell(X,\hat{x})].
\end{equation} 
In a similar manner, for the distributional estimate $\hat{p}_{X}$,
we have the mismatched problem $\hat{p}_{X}^{(q_{X})}=\textrm{argmin\ensuremath{_{\hat{p}_{X}\in\Delta(\mathcal{X})}}}\textrm{E}_{X\sim q_{X}}[\ell(X,\hat{p}_{X})]$.
The difference between the average loss obtained with
the mismatched estimate and the minimum loss $H_{\ell}(X)$ can be
adopted as a measure of the divergence between the two distributions.

For a given loss function $\ell$, this approach yields the following
definition of divergence between two distributions
\begin{equation}
D_{\ell}(p_{X}||q_{X})=\textrm{E}_{X\sim p_{X}}[\ell(X,\hat{x}^{(q_{X})})]-H_{\ell}(p_{X})\label{eq:generalized divergence 1}
\end{equation}
in the case of point estimates, and 
\begin{equation}
D_{\ell}(p_{X}||q_{X})=\textrm{E}_{X\sim p_{X}}[\ell(X,\hat{q}_{X}^{(q_{X})})]-H_{\ell}(p_{X})\label{eq:generalized divergence 1-1}
\end{equation}
for distributional inference. It is noted that the divergence $D_{\ell}(p_{X}||q_{X})$
equals zero if and only if the mismatched estimate performs as well
as the optimal estimate in terms of average loss.

For the quadratic loss, the divergence is given as $D_{\ell_{2}}(p_{X}||q_{X})=(\textrm{E\ensuremath{_{X\sim p_{X}}[X]-}E\ensuremath{_{X\sim q_{X}}[X]}})^{2}$,
which measures the difference in the means of the two pmfs. In the
special case of log-loss, the definition (\ref{eq:generalized divergence 1})
coincides with the conventional KL divergence 
\begin{equation}
D(p_{X}||q_{X})=\textrm{E}_{X\sim p_{X}}\left[\log\frac{p_{X}(X)}{q_{X}(X)}\right].\label{eq:KL divergence}
\end{equation}

By comparing (\ref{eq:generalized divergence 1})-(\ref{eq:generalized divergence 1-1})
with the definition of mutual information (\ref{eq:mutual information}),
it can be seen that the following general relationship holds between the
generalized mutual information and the divergence (\ref{eq:generalized divergence 1})-(\ref{eq:generalized divergence 1-1})
\begin{equation}
I_{\ell}(X;Y)=\textrm{E}_{Y\sim p_{Y}}\left[D_{\ell}(p_{X|Y}||p_{X})\right].
\end{equation}
Hence, the generalized mutual information measures
the average divergence between the conditional pmf $p_{X|Y=y}$ and
the marginal pmf $p_{X}$. 

\emph{Binary Hypothesis Testing}: We now consider the following standard
binary hypothesis testing problem: Given an observation $X$, decide
whether $X$ was generated from pmf $p_{X}$ or from pmf $q_{X}.$
To proceed, we define a decision rule $T(x)$, which should have the
property that it is increasing with the certainty that a value $x$
is generated from $p_{X}$ rather than $q_{X}$. For example, in
practice, one may impose a threshold on the rule $T(x)$ so that,
when $T(x)$ is larger than the threshold, a decision is made that
$X$ was generated from $p_{X}$.

In order to design the decision rule $T(x)$, we again minimize a
loss function or, equivalently, maximize a merit function. For convenience,
here we take the latter approach, and define the problem of maximizing
the merit function
\begin{equation}
\textrm{E}_{X\sim p_{X}}[T(X)]-\textrm{E}_{X\sim q_{X}}[g(T(X))]\label{eq:merit function}
\end{equation}
over the rule $T(x)$, where $g$ is a concave increasing function.
This criterion can be motivated as follows: (\emph{i}) It increases
if $T(x)$ is large, on average, for values of $X$ generated from
$p_{X}$; and (\emph{ii}) it decreases if, upon expectation, $T(x)$
is large for values of $X$ generated from $q_{X}.$ The function
$g$ can be used to define the relative importance of errors made
in favor of one distribution or the other. From this discussion, the
optimal value of (\ref{eq:merit function}) can be taken to be a measure
of the distance between the two pmfs. This yields the following
definition of divergence between two pmfs
\begin{equation}
D_{f}(p_{X}||q_{X})=\max_{T(x)}\textrm{E}_{X\sim p_{X}}[T(X)]-\textrm{E}_{X\sim q_{X}}[g(T(X))],\label{eq:Df}
\end{equation}
where the subscript $f$ will be justified below.

Under suitable differentiability assumptions on function $g$ (see
\cite{fgan} for generalizations), taking the derivative with respect
to $T(x)$ for all $x\in\mathcal{X}$ yields the optimality condition
$g'(T(x))=p_X(x)/q_X(x)$. This relationship reveals the connection between
the optimal detector $T(x)$ and the likelihood ratio $p_X(x)/q_X(x)$.
Plugging this result into (\ref{eq:Df}), it can be directly checked
that the following equality holds \cite{Jordan} 
\begin{equation}
D_{f}(p_X||q_X)=\textrm{E}_{X\sim q_{X}}\left[f\left(\frac{p_{X}(X)}{q_{X}(X)}\right)\right],\label{eq:f divergence}
\end{equation}
where the function $f(x)=g^{*}(x)$ is the convex dual function of
$g(t)$, which is defined as $g^{*}(x)=\sup_{t}\left(xt-g(t)\right)$.
Note that dual function $f$ is always convex \cite{Boyd}.

Under the additional constraint
$f(1)=0$, definition (\ref{eq:f divergence}) describes a large class
of divergence measures parametrized by the convex function $f$, which
are known as $f$-divergences or Ali-Silvey distance measures \cite{Duchi}. Note that the constraint
$f(1)=0$ ensures that the divergence is zero when the pmfs $p_{X}$
and $q_{X}$ are identical. Among their key properties, $f$-divergences satisfy the data processing inequality \cite{Cover,Duchi}.

For example, the choice $g(t)=\exp(t-1)$, which gives the dual convex
$f(x)=x\textrm{log}x$, yields the optimal detector $T(x)=1+\log(p_{X}(x)/q_{X}(x))$
and the corresponding divergence measure (\ref{eq:f divergence})
is the standard KL divergence KL$(p_{X}||q_{X})$ in (\ref{eq:KL divergence}).
As another instance of $f$-divergence, with $g(t)=-\log(2-\exp(t))$
we obtain the optimal detector $T(x)=\log(2p_X(x)/p_X(x)+q_X(x))$, and
$D_{f}(p_{X}||q_{X})$ becomes the Jensen-Shannon divergence. Further examples include the class of $\alpha$-divergences \cite{fgan,Duchi}.

\emph{Remark}: When $p_{X}$ is the empirical distribution of the
data, $q_{X}$ is the empirical distribution obtained from a model
to be learned and $T(x)$ is a parametric detector, problem (\ref{eq:Df})
is a key step of Generative Adversarial Networks (GANs) \cite{GAN}
or, more generally, of f-GANs \cite{fgan}.


The discussion above justified the adoption of the loss function (\ref{eq:Df})
in a heuristic fashion. It is, however, possible to derive formal
relationships between the error probability of binary hypothesis testing
and \emph{f}-divergences \cite{Hero}. 

\subsection*{Conclusions}

In these lecture notes, we have presented an introduction of information
measures in terms of inferential problems, namely estimation for entropy
and conditional entropy, as well as mismatched estimation and binary
hypothesis testing for divergence metrics. This approach allows the definition of general classes of information measures, including as special
cases Shannon's entropy and KL divergence, in an intuitive way that
reveals their operational significance. The variational formulations
that define the information measures as optimal inference problems
can be used to derive learning algorithms, such as in \cite{fgan},
as well as estimates of information measures \cite{Hero,Jordan}. 
\begin{thebibliography}{10}
\bibitem{Cover}T. M. Cover and J. A. Thomas, \emph{Elements of information
theory}, John Wiley \& Sons, 2012.

\bibitem{Bishop}C. M. Bishop, \emph{Pattern recognition and machine
learning,} Springer, 2006.

\bibitem{GrunwaldDawid}P. Grünwald and P. Dawid, ``Game theory,
maximum entropy, minimum discrepancy and robust Bayesian decision
theory,'' \emph{The Annals of Statistics}, vol. 32, no. 4, pp. 1367\textendash 1433,
2004.

\bibitem{Farnia}F. Farnia and D. Tse, ``A minimax approach to supervised
learning,'' in \emph{Proc. Neural Information Processing Systems}
\emph{Conference}, pp. 4240-4248, Barcelona, Spain, Dec. 2016.

\bibitem{Jordan}X. Nguyen, M. J. Wainwright, and M. I. Jordan, \textquotedbl{}Estimating
divergence functionals and the likelihood ratio by convex risk minimization,\textquotedbl{}
\emph{IEEE Trans. Inform. Theory}, vol. 56, no. 11, pp. 5847-5861,
Nov. 2010.

\bibitem{fgan}S. Nowozin, B. Cseke, and R. Tomioka, ``f-GAN: Training
generative neural samplers using variational divergence minimization,''
in \emph{Proc. Neural Information Processing Systems} \emph{Conference},
pp. 4240-4248, Barcelona, Spain, Dec. 2016.

\bibitem{Shannon}C. E. Shannon, ``A mathematical theory of communication,''
\emph{The Bell System Technical Journal}, vol. 27, no. 3, pp. 379-423,
Jul. 1948.

\bibitem{Jiao}J. Jiao, T. A. Courtade, A. No, K. Venkat and T. Weissman,
\textquotedbl{}Information measures: The curious case of the binary
alphabet,\textquotedbl{} \emph{IEEE Trans. Inform. Theory}, vol. 60,
no. 12, pp. 7616-7626, Dec. 2014.

\bibitem{Boyd} S. Boyd and L. Vandenberghe, \emph{Convex optimization}, Cambridge University Press, 2004.

\bibitem{Ruan}J. C. Duchi, K. Khosravi, and F. Ruan, ``Information
measures, experiments, multi-category hypothesis tests, and surrogate
losses,'' arXiv:1603.00126, 2016.

\bibitem{Duchi}J. C. Duchi, \emph{Lecture Notes for Statistics 311/Electrical
Engineering 377}, Stanford University.

\bibitem{GAN}I. Goodfellow, \emph{et al.}, ``Generative
adversarial nets,'' in \emph{Proc. Neural Information Processing
Systems} \emph{Conference}, pp. 2672-2680, Montreal, Canada, Dec.
2014. 

\bibitem{Hero}V. Berisha, A. Wisler, A. Hero, and A. Spanias, ``Empirically
estimable classification bounds based on a nonparametric divergence
measure,'' \emph{IEEE Trans. Signal Proc.}, vol. 64, no. 3, pp. 580-591,
Feb. 2016. 

\end{thebibliography}

\section*{{\small{{AUTHOR}}}}

\textbf{Osvaldo Simeone} is a Professor of Information Engineering with the Centre for Telecommunications Research at the Department of Informatics of King's College London. He received an M.Sc. degree (with honors) and a Ph.D. degree in information engineering from Politecnico di Milano, Milan, Italy, in 2001 and 2005, respectively. He was previously a Professor at the New Jersey Institute of Technology (NJIT). Dr Simeone is a co-recipient of the 2017 JCN Best Paper Award, the 2015 IEEE Communication Society Best Tutorial Paper Award and of the Best Paper Awards of IEEE SPAWC 2007 and IEEE WRECOM 2007. He was awarded a Consolidator grant by the European Research Council (ERC) in 2016. He is a Fellow of the IEEE. 

\end{document}
